# Supplementary material for: Thermal biphotons
Source: arXiv:2008.10636 source file (2022-03-13)
Supplement: Supplementary file 1 [file supp_arxiv.pdf]

**Supplementary information**

Quantum state of thermal biphotons generated via SPDC

In this section, we provide a model for the quantum state of the thermal biphotons generated in our experiment. At the plane of the nonlinear crystal, the quantum state of the generated biphotons is[32]

$$|\psi\rangle = \int d\boldsymbol{q_s} d\boldsymbol{q_i} \nu(\mathbf{q_s} + \boldsymbol{q_i}) \mathrm{A}(\mathbf{q_s}, \mathbf{q_i}) |1_{q_s}, 1_{q_i}\rangle \quad (S1)$$

where $\mathrm{A}(\mathbf{q_s}, \mathbf{q_i}) = sinc\left(\mu_{oo} + l_t(q_{sx} + q_{ix}) + \frac{L}{4k_p}(\boldsymbol{q_s} - \boldsymbol{q_i})^2\right) \exp\left(-il_t(q_{sx} + q_{ix})\right)$ is the phase matching function for a type 1 SPDC process for degenerate photons with a crystal of length $L$, a walk-off length $l_t$ and a pump wavevector $k_p$ inside the crystal. $\mu_{oo}$ is a constant determined by the angle of the nonlinear crystal relative to the pump beam, $\nu(\boldsymbol{q})$ is the angular spectrum of the pump beam, which also includes the normalization constant for the state, and $|1_{q_s}, 1_{q_i}\rangle$ describes a state of signal and idler photons with transverse wavevectors $\boldsymbol{q_s}$ and $\boldsymbol{q_i}$.
Under paraxial propagation of distance $\Delta z$, the quantum state becomes[33]

$$|\psi\rangle = \int d\boldsymbol{q_s} d\boldsymbol{q_i} \nu(\mathbf{q_s} + \boldsymbol{q_i}) \mathrm{A}(\mathbf{q_s}, \mathbf{q_i}) \exp\left(-\frac{i\Delta z}{2k}\left(\boldsymbol{q_i^2} + \boldsymbol{q_s^2}\right)\right) |1_{q_s}, 1_{q_i}\rangle \quad (S2)$$

where $k$ is the wavenumber of the entangled photons.
The state $|\psi\rangle$ can be represented in the spatial domain using the Fourier transform (FT) of the two-photon amplitude $f(\boldsymbol{r_s}, \boldsymbol{r_i}) = FT\left[\nu(\mathbf{q_s} + \boldsymbol{q_i}) \mathrm{A}(\mathbf{q_s}, \mathbf{q_i}) \exp\left(-\frac{i\Delta z}{2k}\left(\boldsymbol{q_i^2} + \boldsymbol{q_s^2}\right)\right)\right]$. Using the polar representation of $f(\boldsymbol{r_s}, \boldsymbol{r_i}) = \sqrt{\mathrm{P}(\mathbf{r_s}, \mathbf{r_i})} \exp\left(\mathrm{i}\left(\Phi(\mathbf{r_s}, \mathbf{r_i})\right)\right)$ we obtain:

$$|\psi\rangle = \int d\mathbf{r_s} d\boldsymbol{r_i} \sqrt{\mathrm{P}(\mathbf{r_s}, \mathbf{r_i})} \exp\left(\mathrm{i}\left(\Phi(\mathbf{r_s}, \mathbf{r_i})\right)\right) |1_{\mathbf{r_s}}, 1_{r_i}\rangle \quad (S3)$$

The normalization of the state, $\langle\psi|\psi\rangle = 1$, thus yields $\int d\boldsymbol{r_s} d\boldsymbol{r_i} P(\boldsymbol{r_s}, \boldsymbol{r_i}) = 1$. Explicit expressions for $\mathrm{P}(\mathbf{r_s}, \mathbf{r_i})$ and $\Phi(\mathbf{r_s}, \mathbf{r_i})$ and their relation to $\Delta z$, $\nu$ and $A$, will be discussed below under the double-Gaussian approximation. For now, we note by inspection of Eq. (S1) that two-photon amplitude is symmetric to the exchange of the signal and idler photons, i.e., $\mathrm{P}(\mathbf{r_s}, \mathbf{r_i}) = \mathrm{P}(\mathbf{r_i}, \mathbf{r_s})$ and $\Phi(\mathbf{r_s}, \mathbf{r_i}) = \Phi(\mathbf{r_i}, \mathbf{r_s})$.
The photons then pass through a rotating thin diffuser, which imposes a time-dependent random phase mask $\phi(\boldsymbol{r})$ onto each of them. The two-photon state is then given by

$$|\psi\rangle = \int d\mathbf{r_s} d\boldsymbol{r_i} \sqrt{\mathrm{P}(\mathbf{r_s}, \mathbf{r_i})} \exp\left(\mathrm{i}\left(\Phi(\mathbf{r_s}, \mathbf{r_i})\right)\right) \exp\left(\mathrm{i}\left(\phi(\mathbf{r_s}) + \phi(\mathbf{r_i})\right)\right) |1_{\mathbf{r_s}}, 1_{r_i}\rangle \quad (S4)$$

Equation (S4) thus describes the quantum state of the signal and idler photons generated via SPDC, undergoing free-space propagation, and finally scattered by a rotating diffuser.

Second-order coherence function

Obtaining the quantum state after the diffuser (Eq. (S4)), we can now proceed to calculate the second-order coherence function. For convenience, we will consider a measurement over a single dimension, yet the same results can be easily extended to two dimensions.

We begin with the calculation of the second-order coherence function

$$g^{(2)}(\Delta\theta) = \frac{\langle\psi|a_s^\dagger(\theta_1)a_i^\dagger(\theta_2)a_i(\theta_2)a_s(\theta_1)|\psi\rangle}{\langle\psi|a_s^\dagger(\theta_1)a_s(\theta_1)|\psi\rangle\langle\psi|a_i^\dagger(\theta_2)a_i(\theta_2)|\psi\rangle} \quad (S5)$$

where $a_{s/i}(\theta) = \sqrt{\frac{k}{2\pi}}\int dr_{s/i}a_{s/i}(r_{s/i})\exp(-ik\theta r_{s/i})$ is the annihilation operator for a signal/idler photon with (paraxial) transverse wavevector $q = k\theta$ at the diffuser's plane.

As the integration time of the measurements is much longer than the typical time scale over which the diffuser rotates, we will be interested in the time-averaged, or equivalently disorder-averaged, results. To this end, it is useful to note that for a diffuser with a sufficiently small correlation width, one can approximate the field-field correlations after the diffuser by[16]

$$\overline{\exp\left(i\big(\phi(r)-\phi(r')\big)\right)} = l\delta(r-r') \quad (S6)$$

where the over-bar denotes temporal averaging and $l$ is a constant with units of length, which depends on the characteristic length scale of the diffuser.

Using this result and the symmetry for signal-idler exchange discussed earlier, we have

$$\begin{aligned}\overline{g^{(2)}(\Delta\theta)} &= \overline{\langle\psi|a_s^\dagger(\theta_1)a_\iota^\dagger(\theta_2)a_\iota(\theta_2)a_s(\theta_1)|\psi\rangle} \\ &= \frac{k^2}{4\pi^2}\int dr_s dr_i dr_s' dr_i' \sqrt{P(r_s,r_i)}\sqrt{P(r_s',r_i')}\exp\Big(\mathrm{i}\big(\Phi(r_s,r_i) \\ &\quad - \Phi(r_s',r_i')\big)\Big)\overline{\exp\Big(\iota\Big(\big(\phi(r_s)+\phi(r_\iota)\big)-\big(\phi(r_s')+\phi(r_\iota')\big)\Big)\Big)}\exp(-ik\theta_1(r_s-r_s') \\ &\quad - ik\theta_2(r_i-r_i')) = \frac{k^2l^2}{4\pi^2}\int dr_s dr_i P(r_s,r_i)\big(1+\exp(-ik\Delta\theta(r_i-\mathrm{r_s})\big) \quad (S7)\end{aligned}$$

And

$$\overline{\langle\psi|a_s^\dagger(\theta_1)a_s(\theta_1)|\psi\rangle} = \overline{\langle\psi|a_i^\dagger(\theta_2)a_i(\theta_2)|\psi\rangle}$$
$$= \frac{k}{2\pi}\int dr_s dr_i dr_s' \sqrt{P(r_s,r_i)}\sqrt{P(r_s{}',r_i)}\,\overline{\exp\left(i\left(\phi(r_s)-\phi(r_s{}')\right)\right)}\exp\left(\mathrm{i}\left(\Phi(r_s,r_i)\right.\right.$$
$$\left.\left.-\Phi(r_s',r_i)\right)\right) exp\left(-ik\theta_1(r_s-r_s')\right) = \frac{kl}{2\pi}\int dr_s dr_i P(r_s,r_i) = \frac{kl}{2\pi} \quad (S8)$$

Yielding

$$\overline{g^{(2)}(\Delta\theta)} = 1 + \int dr_+ dr_- P(r_s,r_i)\exp\left(-i\sqrt{2}k\Delta\theta r_-\right) \quad (S9)$$

where $r_\pm = \frac{r_i \pm r_s}{\sqrt{2}}$.

Defining $h_-(r_-) = \int dr_+ P(r_s,r_i)$ and its Fourier transform $\widetilde{h_-}\left(\sqrt{2}k\Delta\theta\right)$ we have

$$\overline{g^{(2)}(\Delta\theta)} = 1 + \widetilde{h_-}\left(\sqrt{2}k\Delta\theta\right) \quad (S10)$$

From now on, temporal averaging will be implicit in order to simplify the notations.

We note that using the symmetry of $P(r_s,r_i)$, Eq. (S9) can be equivalently written as $g^{(2)}(\Delta\theta) = 1 + \int dr_+ dr_- P(r_s,r_i)\cos\left(\sqrt{2}k\Delta\theta r_-\right)$.

Let us now relate the width of $g^{(2)}(\Delta\theta)$ to the scale $d$, defined in the main text as the average distance between the signal and idler photons at the diffuser's plane. We look at the near-field correlations between the photons $\langle\psi|a_s^\dagger(\mathrm{r_s})a_i^\dagger(r_i)a_i(r_i)a_s(r_s)|\psi\rangle = P(r_s,r_i)$, and define

$$d^2 \equiv \int dr_s dr_i (r_s - r_i)^2 P(r_s,r_i) = \int dr_- 2r_-^2 \int dr_+ P(r_s,r_i) = 2\int dr_- r_-^2 h_-(r_-) \quad (S11)$$

The width of the HBT peak, which is given by the angular width of the Fourier transform of $h_-(r_-)$, therefore scales as $\frac{\lambda}{d}$.

<u>First-order coherence function</u>

To compare Eq. (S10) with the expected result from the Siegert relation, we shall now look at the first-order coherence function, given by

$$g^{(1)}(\Delta\theta) = \frac{\overline{\overline{\langle\psi|a_s^\dagger(\theta_1)a_s(\theta_2)|\psi\rangle}}}{\sqrt{\langle\psi|a_s^\dagger(\theta_1)a_s(\theta_1)|\psi\rangle\langle\psi|a_s^\dagger(\theta_2)a_s(\theta_2)|\psi\rangle}} \quad (S12)$$

Following a similar calculation, we have

$$g^{(1)}(\Delta\theta) = \frac{1}{l}\int dr_s dr_i dr_s' \sqrt{P(r_s,r_i)}\,\overline{\exp\left(i\big(\phi(r_s)-\phi(r_s')\big)\right)}\, exp\left(i\big(\Phi(r_s,r_i) - \Phi(r_s',r_i)\big)\right) exp(-ik\theta_2 r_s + i\theta_1 r_s') = \int dr_s dr_i P(r_s,r_i) exp(-ikr_s\Delta\theta) \quad (S13)$$

As expected from the Van Cittert–Zernike theorem, we obtain that the first order coherence function $g^{(1)}(\Delta\theta)$ at the far-field of the diffuser, is given by the Fourier transform of the single counts distribution at the diffuser's plane $h_s(r_s) \equiv \langle\psi|a_s^\dagger(\mathrm{r_s})a_s(r_s)|\psi\rangle = \int dr_i P(r_s,r_i)$. From this Fourier relation, we conclude that the angular width of $g^{(1)}(\Delta\theta)$ scales as $\frac{\lambda}{D}$, where $D$ is the width of the single photon distribution, defined in the main text as the source size. Comparing this result with the angular width of $g^{(2)}(\Delta\theta)$ found above, we conclude that the Siegert relation can hold only when $\left|\widetilde{h_s}(k\Delta\theta)\right|^2 = \widetilde{h_-}\left(\sqrt{2}k\Delta\theta\right)$. This relation can also be written as $\int dr_s dr_i dr_s' dr_i' P(r_s,r_i)P(r_s',r_i')\exp(-ik(r_s-\mathrm{r}_s')\Delta\theta) = \int dr_s dr_i P(r_s,r_i)\exp(-ik\Delta\theta(r_s-r_i))$. For a separable state, $P(r_s,r_i) = P_1(r_s)P_1(r_i)$, and therefore $\int dr_i dr_i' P(r_s,r_i)P(r_s',r_i') = P(r_s,r_s')$. We thus get that for a separable pure state the Siegert relation indeed holds.

For an inseparable state, although the Siegert relation does not necessarily hold, a Siegert-like relation of the form $g^{(2)}(\Delta\theta) = 1 + \left|\tilde{f}(k\Delta\theta)\right|^2$ can still be obtained, where $\tilde{f}(k\Delta\theta) = \sqrt{\widetilde{h_-}\left(\sqrt{2}k\Delta\theta\right)}$ depends on $d$ rather than $D$ for the standard Siegert relation. We therefore obtain a relation between the width of the HBT peak and the size of the equivalent two-photon emitter, rather than the total size of the source.

Density matrix formalism

In the previous sections, we used a pure-state formalism, and performed the temporal averaging when calculating the expectation values for the coherence functions. Alternatively, we can work in the density matrix formalism, and perform the temporal averaging (disorder averaging) on the state itself. The mixed state formalism is valid when the integration time of the measurement is much longer than the correlation time of the rotating diffuser.

We write

$$\hat{\rho} = \int dr_s dr_i dr_s' dr_i' \sqrt{P(r_s,r_i)}\sqrt{P(r_s',r_i')}\exp\left(\mathrm{i}\big(\Phi(r_s,r_i) - \Phi(r_s',r_i')\big)\right)\overline{\exp\left(i\left(\big(\phi(r_s)+\phi(r_i)\big) - \big(\phi(r_s')+\phi(r_i')\big)\right)\right)}\,|1_{r_s},1_{r_i}\rangle\langle 1_{r_s'},1_{r_i'}| = \int dr_s dr_i \tilde{P}(r_s,r_i)\left(|1_{r_s},1_{r_i}\rangle\langle 1_{r_s},1_{r_i}| + |1_{r_s},1_{r_i}\rangle\langle 1_{r_i},1_{r_s}|\right) \quad (S14)$$

where $\tilde{P}(r_s, r_i) = l^2 P(r_s, r_i)$. Of course, all results presented earlier can be equivalently obtained using this formalism as well.

Double-Gaussian approximation

To get explicit and simple expressions for the first- and second-order coherence functions we use the double-Gaussian approximation for the quantum state of SPDC[32]

$$|\psi\rangle_{DG} \propto \int dq_s dq_i \exp\left(-\frac{(q_s+q_i)^2}{\sigma_1^2}\right)\exp\left(-\frac{(q_s-q_i)^2}{\sigma_2^2}\right)|1_{q_s}, 1_{\mathrm{q_i}}\rangle \qquad (S15)$$

where $\sigma_1$ is related the waist of the pump beam at the plane of the crystal by $\sigma_1 = \frac{2}{\sigma_p}$, and $\sigma_2 = \sqrt{\frac{4k_p}{L}}$ where $L$ is the length of the nonlinear crystal and $k_p$ is the wavevector of the pump beam inside the crystal.

In this case, one can easily see that $P(r_s, r_i) \propto exp\left(-\frac{r_+^2}{2\sigma_+{}^2(\Delta z)}\right) exp\left(-\frac{r_-^2}{2\sigma_-{}^2(\Delta z)}\right)$, where $\sigma_-(\Delta z) = \sqrt{2\left(\frac{1}{\sigma_2^2}+\frac{\Delta z^2\sigma_2^2}{16k^2}\right)}$ and $\sigma_+(\Delta z) = \sqrt{2\left(\frac{1}{\sigma_1^2}+\frac{\Delta z^2\sigma_1^2}{16k^2}\right)}$, and identify $d = \sqrt{2}\sigma_-(\Delta z)$ and $D = \frac{\sqrt{\sigma_+{}^2(\Delta z)+\sigma_-{}^2(\Delta z)}}{\sqrt{2}}$.

Substituting the above expression for $P(r_s, r_i)$ into the first- and second-order coherence functions calculated earlier (Eq. (S10) and (S13)) yields

$$g_{DG}^{(2)}(\Delta\theta) = 1 + \exp\left(-\frac{\sigma_-{}^2(\Delta z)\left(\sqrt{2}k\Delta\theta\right)^2}{2}\right) = 1 + \exp\left(-\frac{d^2(k\Delta\theta)^2}{2}\right) \qquad (S16)$$

$$\left|g_{DG}^{(1)}(\Delta\theta)\right|^2 = exp\left(-\frac{\left(\sigma_+{}^2(\Delta z)+\sigma_-^2(\Delta z)\right)(k\Delta\theta)^2}{2}\right) = exp(-D^2(k\Delta\theta)^2) \qquad (S17)$$

Indeed, the Siegert relation, $g_{DG}^{(2)}(\Delta\theta) = 1 + \left|g_{DG}^{(1)}(\Delta\theta)\right|^2$, only holds when $\sigma_+(\Delta z) = \sigma_-(\Delta z)$, which is always true for a separable state, i.e. for $\sigma_1 = \sigma_2$. Thus, in the context of SPDC under the double-Gaussian approximation, spatial entanglement is required for the breaking of the Siegert relation.

To quantify the role of entanglement in the breaking of the Siegert relation, we can look at the ratio of area of the HBT peak and the area of $\left|g_{DG}^{(1)}(\Delta\theta)\right|^2$, $W_r = \frac{\left(\sigma_+{}^2(\Delta z)+\sigma_-^2(\Delta z)\right)}{2\sigma_-{}^2(\Delta z)} =$

$\frac{1}{2}\left(\frac{\frac{1}{\sigma_1^2}+\frac{\Delta z^2\sigma_1^2}{16k^2}}{\frac{1}{\sigma_2^2}+\frac{\Delta z^2\sigma_2^2}{16k^2}}+1\right)$. Assuming high spatial entanglement, the Schmidt number under the double-Gaussian approximation is given by $K \approx \frac{1}{4}\frac{\sigma_2^2}{\sigma_1^2}$[32]. Thus, for $\Delta z = 0$, we have $W_r \approx 2\left(K+\frac{1}{4}\right)$ and a direct relation to the entanglement in the state is observed. We note that for large distances, where $\Delta z \gg \frac{k}{\sigma_1^2}$ and $\Delta z \gg \frac{k}{\sigma_2^2}$, we have $W_r \approx \frac{1}{8}\left(\frac{1}{K}+4\right)$, and the width of the HBT peak can be smaller by up to a factor of $\sqrt{2}$ compared with the width of $\left|g_{DG}^{(1)}(\Delta\theta)\right|^2$. Experimental demonstration of this result is out of the scope of the current work, yet it could be an interesting direction for future studies.

Recovering Siegert's relation

We reproduce the standard HBT effect, by considering the case where the size of the two-photon emitters is similar to the size of the source, $d \approx D$. This is obtained for $\Delta z = 100mm$ in our experiment (Fig. S1, black dots). As expected, an HBT peak is observed near $\Delta\theta = 0$, where the reduced peak height is due to its convolution with the $100\mu m$ wide detectors. In contrast with the results for $D \approx 2d$ presented in the main text (Fig. S1, blue), the Siegert relation approximately holds in this case.

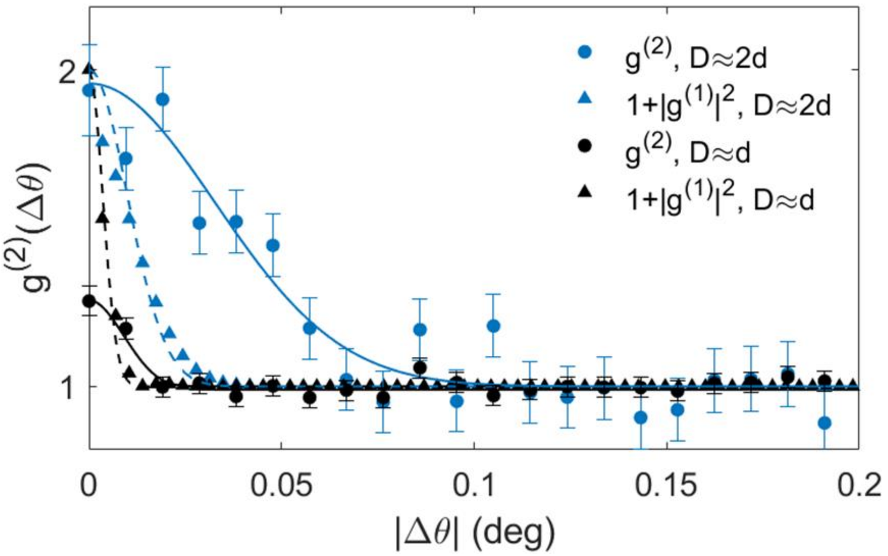


Figure S1: Second-order $g^{(2)}(\Delta\theta)$ and first-order $g^{(1)}(\Delta\theta)$ coherence measurements of thermal biphotons. The data for the black and blue curves is taken with $\Delta z = 100mm$ ($d \approx D$) and $\Delta z = 35mm$ ($D \approx 2d$, as presented in the main text), respectively. Fits based on the double-Gaussian model are plotted in dashed and solid curves for the first- and second-order coherence functions, respectively. For $\Delta z = 35mm$ we obtain $d = 230 \pm 16\ \mu m, D = 525 \pm 2\ \mu m$, and for $\Delta z = 100mm$, $d = 1600 \pm 100\ \mu m, D = 1470 \pm 15\ \mu m$.
